# Supplementary material for: Learning to combine primitive skills: A step towards versatile robotic manipulation
Source: arXiv:1908.00722 source file (2020-06-20)
Supplement: Supplementary file 1 [file appendix.tex]

\section{Appendix}

We present additional qualitative results for the RLBC approach on the real robot with policies that have been trained in simulation, as in the main paper. Section~\ref{sec:qualitative} describes and illustrates examples of UR5-Bowl and UR5-Breakfast policies, also shown in the video. We demonstrate robot behavior while the robot is facing the challenges of previously unseen objects, dynamic changes of object locations and occlusions. We also illustrate feature map activations of the network providing better understanding of learned policies in Section~\ref{sec:activations}.

\subsection{Qualitative results}
% \vspace{-.1cm}
\label{sec:qualitative}

\paragraph{UR5-Bowl: Multiple objects.} We experiment with the RLBC policy trained in the UR5-Bowl environment. Once the robot succeeds to place a cube in the bowl, we put another cube on the table and let the policy continue, see Figure~\ref{fig:ur5-bowl-2cubes}. While the UR5-Bowl policy has been trained to handle one cube only, it automatically generalizes to multiple cubes when run in a loop.

\begin{figure}[h!]
   \centering
        % trim <left> <lower> <right> <upper>
        \includegraphics[trim={50 20 50 40},clip,width=0.22\textwidth]{imgs/ur5-bowl-2cubes_01.jpg}
        \includegraphics[trim={50 20 50 40},clip,width=0.22\textwidth]{imgs/ur5-bowl-2cubes_02.jpg}
        \includegraphics[trim={50 20 50 40},clip,width=0.22\textwidth]{imgs/ur5-bowl-2cubes_03.jpg}
        \includegraphics[trim={50 20 50 40},clip,width=0.22\textwidth]{imgs/ur5-bowl-2cubes_04.jpg}
   \caption{RLBC approach for UR5-Bowl with two cubes.\vspace{-.1cm}}
\label{fig:ur5-bowl-2cubes}
\end{figure}

\paragraph{UR5-Bowl: Previously unseen objects.} We further test the RLBC UR5-Bowl policy in the presence of previously unseen objects. While the policy has been trained to manipulate cubes of different sizes (see Section~5.1), we observe its robustness to other object shapes. As shown in Figure~\ref{fig:ur5-bowl-newobj}, the policy successfully grasps and places into a bowl real objects, such as apples, oranges, lemons, and toys. Notably, in cases of failing to grasps an object, the robot automatically recovers and completes the task. This behavior comes naturally from our RLBC master policy that has learned to adapt the sequence of skills given current observations of the scene.

\begin{figure}[h!]
   \centering
        % trim <left> <lower> <right> <upper>
        \includegraphics[trim={50 20 50 40},clip,width=0.22\textwidth]{imgs/ur5-bowl-newobj_01.jpg}
        \includegraphics[trim={50 20 50 40},clip,width=0.22\textwidth]{imgs/ur5-bowl-newobj_02.jpg}
        \includegraphics[trim={50 20 50 40},clip,width=0.22\textwidth]{imgs/ur5-bowl-newobj_05.jpg}
        \includegraphics[trim={50 20 50 40},clip,width=0.22\textwidth]{imgs/ur5-bowl-newobj_06.jpg}\smallskip \\
        \includegraphics[trim={50 20 50 40},clip,width=0.22\textwidth]{imgs/ur5-bowl-newobj_07.jpg}
        \includegraphics[trim={50 20 50 40},clip,width=0.22\textwidth]{imgs/ur5-bowl-newobj_08.jpg}
        \includegraphics[trim={50 20 50 40},clip,width=0.22\textwidth]{imgs/ur5-bowl-newobj_03.jpg}
        \includegraphics[trim={50 20 50 40},clip,width=0.22\textwidth]{imgs/ur5-bowl-newobj_04.jpg}
   \caption{RLBC approach for UR5-Bowl with previously unseen objects.\vspace{-.5cm}}
\label{fig:ur5-bowl-newobj}
\end{figure}

\paragraph{UR5-Breakfast: New object instances.}

To enable generalization of learned policies to new object instances, our UR5-Breakfast environment contains cups, bottles and bowls of different shapes from ShapeNet (see Section~5.1). During testing we run the learned RLBC UR5-Breakfast policy on a real robot and experiment with instances of bottles and cups unseen during training. Figure~\ref{fig:ur5-breakfast-newobj} demonstrates successful executions of the RLBC UR5-Breakfast policy in scenes with significant variations in object shapes, for example, using a wine glass instead of a cup. 

\begin{figure}[h!]
   \centering
        % trim <left> <lower> <right> <upper>
        \includegraphics[trim={40 20 50 30},clip,width=0.22\textwidth]{imgs/ur5-breakfast-newobj_01.jpg}
        \includegraphics[trim={40 20 50 30},clip,width=0.22\textwidth]{imgs/ur5-breakfast-newobj_02.jpg}
        \includegraphics[trim={40 20 50 30},clip,width=0.22\textwidth]{imgs/ur5-breakfast-newobj_03.jpg}
        \includegraphics[trim={40 20 50 30},clip,width=0.22\textwidth]{imgs/ur5-breakfast-newobj_04.jpg}
   \caption{RLBC approach for UR5-Breakfast with previously unseen object instances.\vspace{-.5cm}}
\label{fig:ur5-breakfast-newobj}
\end{figure}

\paragraph{UR5-Breakfast: Dynamic changes of object location.}

Our BC skills make decisions at every time-step and, hence, can instantly adapt to changing conditions of the scene. We verify this by varying object positions during grasping attempts of the RLBC UR5-Breakfast policy. Figure~\ref{fig:ur5-breakfast-reactive} illustrates the reactive behavior of the robot grasping a cup that is being simultaneously moved by the person. The cup is successfully grasped after multiple changes of its position.

\begin{figure}[h!]
   \centering
        % trim <left> <lower> <right> <upper>
        \includegraphics[trim={20 0 40 10},clip,width=0.22\textwidth]{imgs/ur5-breakfast-reactive_02.jpg}
        \includegraphics[trim={20 0 40 10},clip,width=0.22\textwidth]{imgs/ur5-breakfast-reactive_03.jpg}
        \includegraphics[trim={20 0 40 10},clip,width=0.22\textwidth]{imgs/ur5-breakfast-reactive_04.jpg}
        \includegraphics[trim={20 0 40 10},clip,width=0.22\textwidth]{imgs/ur5-breakfast-reactive_05.jpg}
   \caption{RLBC approach for UR5-Breakfast with dynamic changes of object locations.\vspace{-.5cm}}
\label{fig:ur5-breakfast-reactive}
\end{figure}

\paragraph{UR5-Breakfast: Occlusion.}

Another example of the instant re-planning by our RLBC policy is demonstrated in Figure~\ref{fig:ur5-breakfast-occlusion}. While the robot approaches an object, we temporary occlude the object and disrupt the executing BC skill. Given the hierarchical nature of our RLBC approach, the RL master is able to recover from this failure by starting another skill that leads to the completion of the task. More precisely, when the bottle gets occluded in the example of Figure~\ref{fig:ur5-breakfast-occlusion}, the robot changes its strategy and decides to grasp and pour from a cup. Once the occlusion is removed, the robot automatically resumes and completes the task by grasping and pouring from the bottle.

\begin{figure}[h!]
   \centering
        % trim <left> <lower> <right> <upper>
        \includegraphics[trim={0 0 60 10},clip,width=0.24\textwidth]{imgs/ur5-breakfast-occlusion_01.jpg}
        \includegraphics[trim={0 0 35 10},clip,width=0.24\textwidth]{imgs/ur5-breakfast-occlusion_02.jpg}
        \includegraphics[trim={0 0 48 10},clip,width=0.24\textwidth]{imgs/ur5-breakfast-occlusion_03.jpg}\\
        \includegraphics[trim={0 0 45 10},clip,width=0.24\textwidth]{imgs/ur5-breakfast-occlusion_04.jpg}
        \includegraphics[trim={0 0 50 10},clip,width=0.24\textwidth]{imgs/ur5-breakfast-occlusion_05.jpg}
        \includegraphics[trim={0 0 50 10},clip,width=0.24\textwidth]{imgs/ur5-breakfast-occlusion_06.jpg}
   \caption{RLBC UR5-Breakfast policy executed in a robot scene with a temporary occluded bottle.\vspace{-.5cm}}
\label{fig:ur5-breakfast-occlusion}
\end{figure}

% \newpage

\paragraph{UR5-Breakfast: Failure case for BC-ordered.}

Finally, we demonstrate the advantage of RLBC compared to the "BC-ordered" baseline with a fixed order of skills. For the UR5-Breakfast environment we define the order of skills for the BC-ordered policy as 1.~"go to the cup", 2.~"grasp the object and pour it to the bowl", 3.~"release the object", 4.~"go to the bottle", 5.~"grasp the object and pour it to the bowl", 6.~"release the object". While this policy succeeds in many cases, the near placement of objects presents a source of problems. Figure~\ref{fig:ur5-breakfast-bc-failure} shows an example scene with a cup and a bottle being near to each other while the cup is placed in front of the bottle. As the BC-ordered policy above is pre-programmed to grasp the cup first, the execution of this policy results in a collision between a gripper and a bottle, followed by the failure of the task. Notably, our RLBC policy learns to select the order of objects for grasping such as to avoid failures of the task. Hence, the RLBC automatically learns to avoid collisions without the need of specific intermediate rewards. This advantage of RLBC is demonstrated by quantitative results in Table~3 and by qualitative results in the last part of the video.

\begin{figure}[h!]
   \centering
        % trim <left> <lower> <right> <upper>
        \includegraphics[trim={20 0 40 10},clip,width=0.22\textwidth]{imgs/ur5-breakfast-bc-failure_01.jpg}
        \includegraphics[trim={20 0 40 10},clip,width=0.22\textwidth]{imgs/ur5-breakfast-bc-failure_02.jpg}
        \includegraphics[trim={20 0 40 10},clip,width=0.22\textwidth]{imgs/ur5-breakfast-bc-failure_03.jpg}
        \includegraphics[trim={20 0 40 10},clip,width=0.22\textwidth]{imgs/ur5-breakfast-bc-failure_04.jpg}
   \caption{Illustration of a failure case for the BC-ordered approach for UR5-Breakfast with close by objects.\vspace{-.5cm}}
\label{fig:ur5-breakfast-bc-failure}
\end{figure}

\subsection{Feature map activations}
\label{sec:activations}

The RLBC policy uses no explicit representation of scenes, for example in terms of categories and locations of objects. Some interpretation of learned policies, however, can be obtained by examining spatial activations of the neural network at intermediate network layers. Figure~\ref{fig:ur5-breakfast-heatmab} shows silency maps of an RLBC policy highlighting which parts of the image the agents concentrates on. The silency maps are computed as activations of convolutional feature maps obtained from last layers of $CNN(\theta)$ and $CNN(\eta^i), i=1,\ldots,K$  (see Figure~1), averaged over all channels and layers. The resulting heatmaps are shown for different stages of the UR5-Breakfast task. Interestingly, while grasping and moving the bottle, the network generates highest activations around the bottle and the gripper, while ignoring other objects. When releasing the bottle, however, high activations are also observed around the cup. The attention to the cup might be explained by the need of avoiding collisions when placing the bottle on the table. Note, that we provide no intermediate rewards to RL, however, RL learns to avoid collisions since collisions imply failures of the final task and, hence, no final positive reward during training. Once the bottle is placed on the table, activations become low for the bottle, while the heatmap obtains maximum values for the manipulated cup. Observations of such feature maps have been useful in our work to identify certain cases of failures. We believe feature map activations are a useful tool to interpret learned policies. More examples of feature map activations are available in the video. 

\begin{figure}[h!]
   \centering
   \begin{tabular}{c}
        % trim <left> <lower> <right> <upper>
        {\em grasping bottle} \\ 
        \includegraphics[trim={0 13 0 0},clip,width=0.19\textwidth]{imgs/ur5-breakfast-heatmap_01.jpg}
        \includegraphics[trim={0 0  0 0},clip,width=0.275\textwidth]{imgs/ur5-breakfast-heatmap_01orig.jpg}\\
        {\em moving bottle}\\
        \includegraphics[trim={0 13 0 0},clip,width=0.19\textwidth]{imgs/ur5-breakfast-heatmap_02.jpg}
        \includegraphics[trim={0 0  0 0},clip,width=0.275\textwidth]{imgs/ur5-breakfast-heatmap_02orig.jpg}\\
        {\em pouring from bottle}\\
        \includegraphics[trim={0 13 0 0},clip,width=0.19\textwidth]{imgs/ur5-breakfast-heatmap_03.jpg}
        \includegraphics[trim={0 0  0 0},clip,width=0.275\textwidth]{imgs/ur5-breakfast-heatmap_03orig.jpg}\\
        {\em releasing bottle}\\
        \includegraphics[trim={0 13 0 0},clip,width=0.19\textwidth]{imgs/ur5-breakfast-heatmap_04.jpg}
        \includegraphics[trim={0 0  0 0},clip,width=0.275\textwidth]{imgs/ur5-breakfast-heatmap_04orig.jpg}\\
        {\em grasping cup}\\
        \includegraphics[trim={0 13 0 0},clip,width=0.19\textwidth]{imgs/ur5-breakfast-heatmap_05.jpg}
        \includegraphics[trim={0 0  0 0},clip,width=0.275\textwidth]{imgs/ur5-breakfast-heatmap_05orig.jpg}\\
        {\em pouring from cup}\\
        \includegraphics[trim={0 13 0 0},clip,width=0.19\textwidth]{imgs/ur5-breakfast-heatmap_06.jpg}
        \includegraphics[trim={0 0  0 0},clip,width=0.275\textwidth]{imgs/ur5-breakfast-heatmap_06orig.jpg}\\
    \end{tabular}
   \caption{Left: Feature map activations of the RLBC  UR5-Breakfast policy are overlayed on the input depth images. Right: corresponding frames taken from a different viewpoint.}
\label{fig:ur5-breakfast-heatmab}
\end{figure}
